# Supplementary material for: A Training-free Sub-quadratic Cost Transformer Model Serving Framework With Hierarchically Pruned Attention
Source: arXiv:2406.09827 source file (2025-01-23)
Supplement: Supplementary file 1 [file hip_theory_appendix_kldivergence_othermodels.tex]

\begin{figure}[t]
\vspace{.5em}%
\centering%
\begin{subfigure}[b]{\textwidth}
    \includegraphics[width=\linewidth, trim = 0mm 0mm 0mm 0mm, clip]{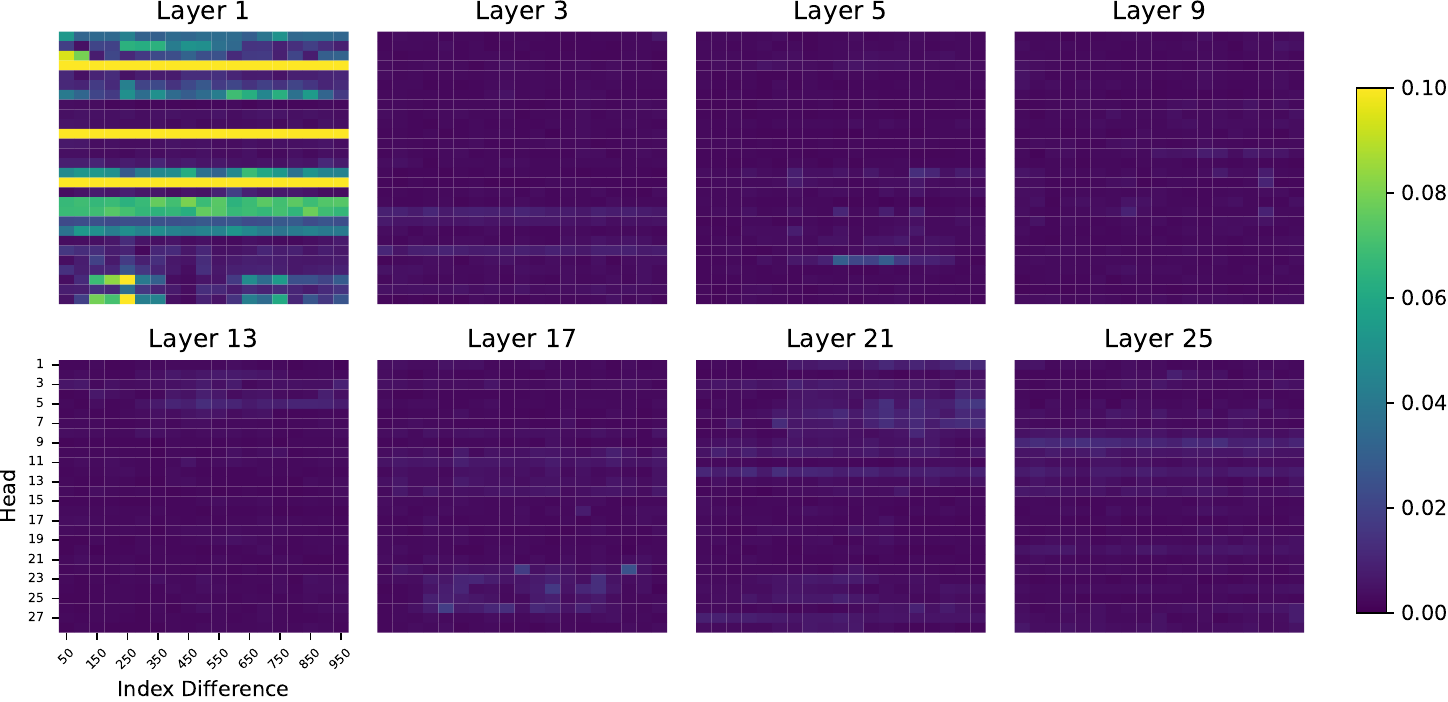}
    \caption{{\color{blue}Qwen2 7B Model.}}
\end{subfigure}
\begin{subfigure}[b]{\textwidth}
    \includegraphics[width=\linewidth, trim = 0mm 0mm 0mm 0mm, clip]{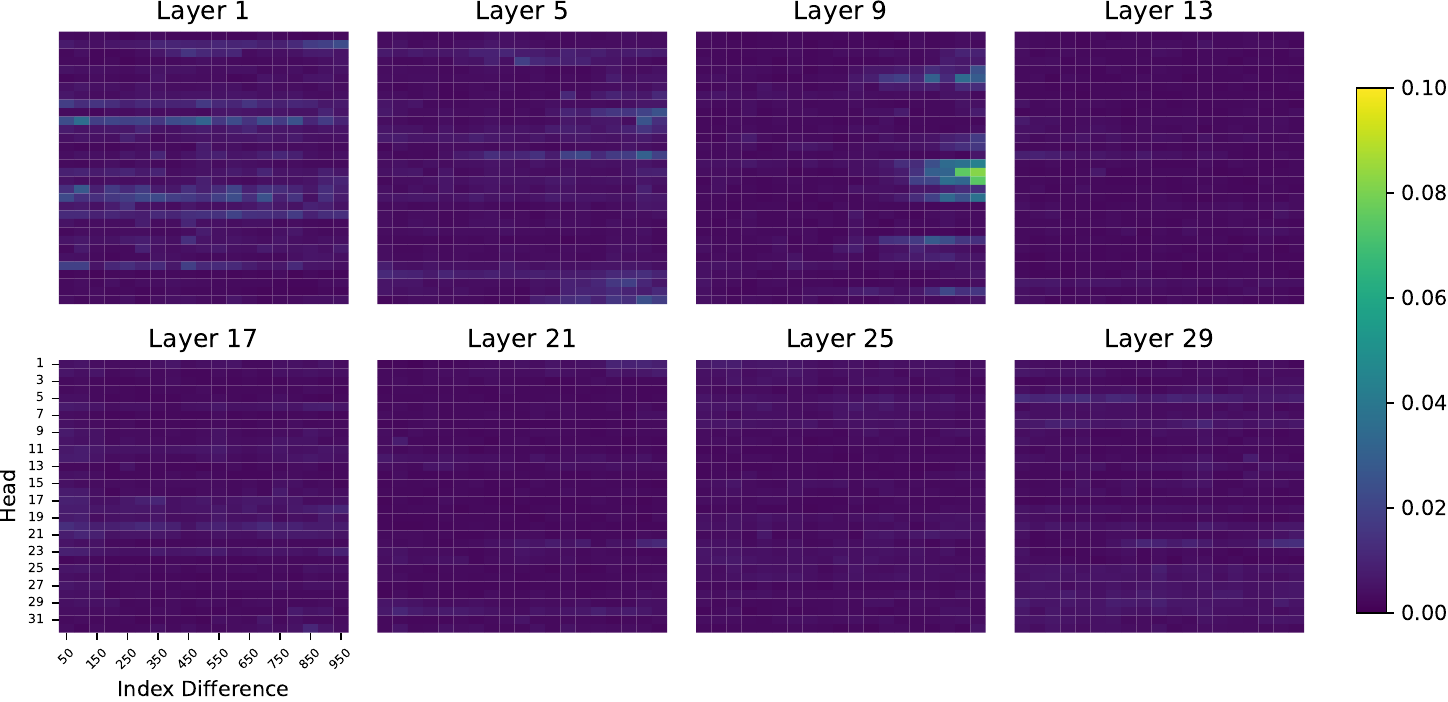}
    \caption{{\color{blue}Exaone 3.0 7.8B Model.}}
\end{subfigure}
\captionof{figure}{\color{blue}\textbf{KL Divergence of Other Models.} The above figures display the KL Divergences between $\delta_\Delta$ and its fitted normal distributions of various layers for the Qwen2 and Exaone models, similar to \Cref{fig:appendix_attn_kldivergence}. The Wikitext2 dataset was used as input for the models.
}
\label{fig:appendix_attn_kldivergence_othermodels}%
\vspace{.5em}%
\end{figure}
