# Supplementary material for: A Training-free Sub-quadratic Cost Transformer Model Serving Framework With Hierarchically Pruned Attention
Source: arXiv:2406.09827 source file (2025-01-23)
Supplement: Supplementary file 2 [file hip_theory_appendix_normal_othermodels.tex]

\begin{figure}[t]
\centering%

\captionof{figure}{{\color{blue}\textbf{Distribution of $\delta_\Delta$.} The above figures show the distributions of $\delta_\Delta$ for $\Delta$ values 200, 400, 600, and 800 for the Qwen2 7B and Exaone 3.0 7.8B models. The values were sampled from the $6^\textbf{th}$ attention head of the $9^\textbf{th}$ layer in the Qwen2 model, and the $6^\textbf{th}$ head of the $13^\textbf{th}$ layer in the Exaone model. The Wikitext2 dataset was used as input, similarly to \Cref{fig:appendix_attn_normal_distribution}.}
}%
\label{fig:appendix_attn_normal_distribution_others}%
\vspace{.5em}
\end{figure}
