# Supplementary material for: A Training-free Sub-quadratic Cost Transformer Model Serving Framework With Hierarchically Pruned Attention
Source: arXiv:2406.09827 source file (2025-01-23)
Supplement: Supplementary file 3 [file hip_theory_appendix_sigma_othermodels.tex]

\begin{figure}[t]
%\vspace{-.5em}%
\centering%
\begin{subfigure}[b]{\textwidth}
    \includegraphics[width=\linewidth, trim = 0mm 0mm 0mm 0mm, clip]{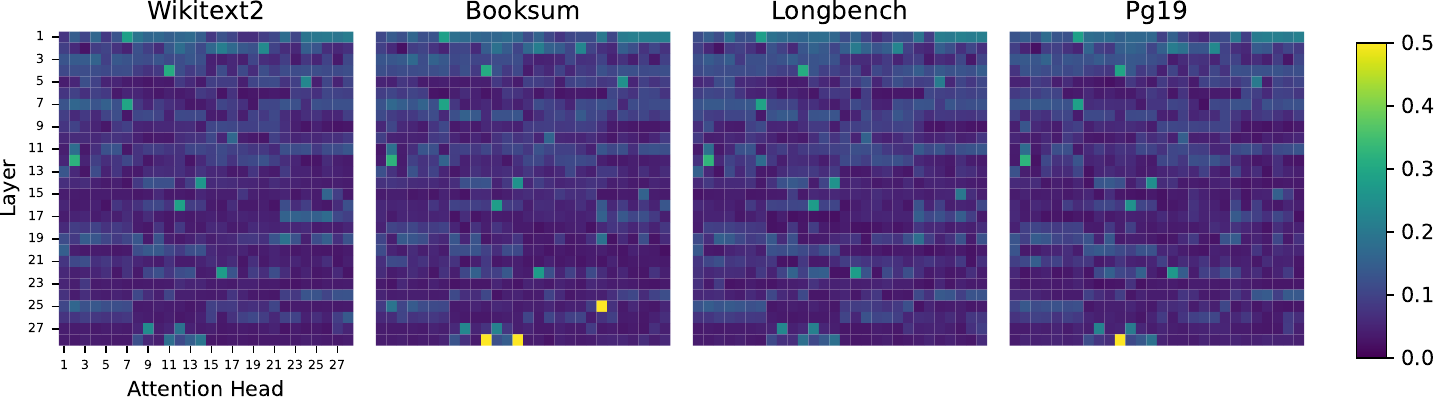}
    \caption{\color{blue}Qwen2 7B Model.}
\end{subfigure}
\begin{subfigure}[b]{\textwidth}
    \includegraphics[width=\linewidth, trim = 0mm 0mm 0mm 0mm, clip]{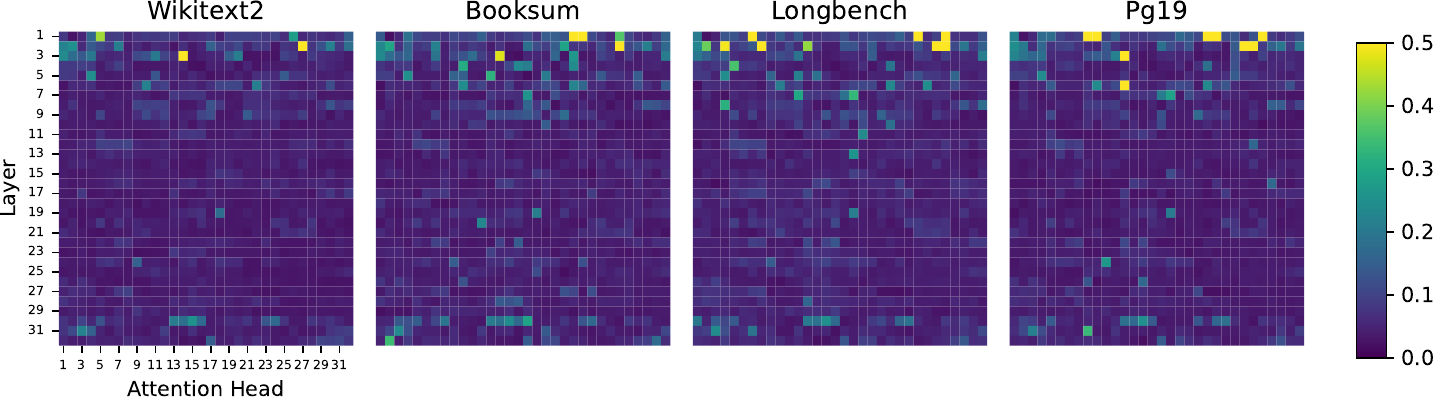}
    \caption{\color{blue}Exaone 3.0 7.8B Model.}
\end{subfigure}
\vspace{-2em}%
\captionof{figure}{\color{red}\textbf{NRMSE Colormaps for Qwen2 and Exaone Models.} The above figures show the NRMSE errors of fitting the $\sigma(\Delta)$ function to a logarithmic function as a heatmap, similarly to \Cref{fig:appendix_sigma}. 
}
\label{fig:appendix_sigma_others}%
\end{figure}
