# Supplementary material for: A Training-free Sub-quadratic Cost Transformer Model Serving Framework With Hierarchically Pruned Attention
Source: arXiv:2406.09827 source file (2025-01-23)
Supplement: Supplementary file 4 [file hip_theory_appendix_sigmagraph_othermodels.tex]

\begin{figure}[t]
% \begin{subfigure}[t]{\textwidth}
%     \centering
%     \begin{minipage}[b]{0.24\textwidth}
%         \centering
%         \includegraphics[width=\textwidth]{figures/appendix_sigma_layer12_head4_qwen2.pdf}
%     \end{minipage}%
%     \begin{minipage}[b]{0.24\textwidth}
%         \centering
%         \includegraphics[width=\textwidth]{figures/appendix_sigma_layer12_head8_qwen2.pdf}
%     \end{minipage}%
%     \begin{minipage}[b]{0.24\textwidth}
%         \centering
%         \includegraphics[width=\textwidth]{figures/appendix_sigma_layer12_head12_qwen2.pdf}
%     \end{minipage}%
%     \begin{minipage}[b]{0.24\textwidth}
%         \centering
%         \includegraphics[width=\textwidth]{figures/appendix_sigma_layer12_head16_qwen2.pdf}
%     \end{minipage}\\[1ex]
    
%     \begin{minipage}[b]{0.24\textwidth}
%         \centering
%         \includegraphics[width=\textwidth]{figures/appendix_sigma_layer12_head20_qwen2.pdf}
%     \end{minipage}%
%     \begin{minipage}[b]{0.24\textwidth}
%         \centering
%         \includegraphics[width=\textwidth]{figures/appendix_sigma_layer12_head24_qwen2.pdf}
%     \end{minipage}%
%     \begin{minipage}[b]{0.24\textwidth}
%         \centering
%         \includegraphics[width=\textwidth]{figures/appendix_sigma_layer12_head28_qwen2.pdf}
%     \end{minipage}%
%     \caption{\color{blue} Qwen2 7B Model.}
% \end{subfigure}

% \begin{subfigure}[t]{\textwidth}
%     \centering
%     \begin{minipage}[b]{0.24\textwidth}
%         \centering
%         \includegraphics[width=\textwidth]{figures/appendix_sigma_layer16_head4_exaone.pdf}
%     \end{minipage}%
%     \begin{minipage}[b]{0.24\textwidth}
%         \centering
%         \includegraphics[width=\textwidth]{figures/appendix_sigma_layer16_head8_exaone.pdf}
%     \end{minipage}%
%     \begin{minipage}[b]{0.24\textwidth}
%         \centering
%         \includegraphics[width=\textwidth]{figures/appendix_sigma_layer16_head12_exaone.pdf}
%     \end{minipage}%
%     \begin{minipage}[b]{0.24\textwidth}
%         \centering
%         \includegraphics[width=\textwidth]{figures/appendix_sigma_layer16_head16_exaone.pdf}
%     \end{minipage}\\[1ex]
    
%     \begin{minipage}[b]{0.24\textwidth}
%         \centering
%         \includegraphics[width=\textwidth]{figures/appendix_sigma_layer16_head20_exaone.pdf}
%     \end{minipage}%
%     \begin{minipage}[b]{0.24\textwidth}
%         \centering
%         \includegraphics[width=\textwidth]{figures/appendix_sigma_layer16_head24_exaone.pdf}
%     \end{minipage}%
%     \begin{minipage}[b]{0.24\textwidth}
%         \centering
%         \includegraphics[width=\textwidth]{figures/appendix_sigma_layer16_head28_exaone.pdf}
%     \end{minipage}%
%     \begin{minipage}[b]{0.24\textwidth}
%         \centering
%         \includegraphics[width=\textwidth]{figures/appendix_sigma_layer16_head32_exaone.pdf}
%     \end{minipage}
%     \caption{\color{blue} Exaone 3.0 7.8B Model.}
% \end{subfigure}

\captionof{figure}{\color{red}\textbf{Plots of $\sigma(\Delta$) and their Normalized Root Mean Squared Error.} The above figures show plots of $\sigma(\Delta)$, and the NRMSE fitting errors for the Qwen2 and Exaone models, similarly to \Cref{fig:appendix_sigma_plots}. For the above plots, the 12th layer of the Qwen2 model and the 16th layer of the Exaone model were used. The Wikitext2 dataset was used as the input for these models.
}%
\label{fig:appendix_sigma_plots_othermodels}
\end{figure}
