# Supplementary material for: A Training-free Sub-quadratic Cost Transformer Model Serving Framework With Hierarchically Pruned Attention
Source: arXiv:2406.09827 source file (2025-01-23)
Supplement: Supplementary file 5 [file appendix_ensemble.tex]

%%%%%%%%%%%%%%%%%%%%%%%%%%%%%%%%%%%%%%%%%%%%%%%%%%%%%%%%%%%%%%%%%%
% ** section header is in 7_appendix.tex ** 
% DO NOT PUT SECTION IN THIS FILE
%%%%%%%%%%%%%%%%%%%%%%%%%%%%%%%%%%%%%%%%%%%%%%%%%%%%%%%%%%%%%%%%%

% Instead of generating multiple individual masks like an ensemble, each with different branching in a particular iteration, we can achieve a similar effect by diversifying the tree branching beyond that of a binary tree, akin to an n-beam search. 
% This approach allows for multi-branching with a single HiP execution while eliminating the need to generate multiple HiP masks as required in the ensemble method. 
% Moreover, unlike the ensemble method, where each mask includes some overlapping indices, the multi-branch approach ensures a different selection of indices for each branch. 
% As a result, we think the multi-branch approach could reduce the ensemble method's memory usage and computational cost while potentially offering higher performance.
% Although multi-branching incurs a higher cost than HiP, we hope to balance the performance-cost trade-off by adjusting either the number of branches or the iteration point at which multi-branching is applied. 
% This would likely enable comparable performance at a reduced cost compared to the HiP with dense layers.
